# Supplementary material for: FedSAE: A Novel Self-Adaptive Federated Learning Framework in Heterogeneous Systems
Source: arXiv:2104.07515 source file (2021-04-15)
Supplement: Supplementary file 1 [file Appendix.tex]

\section{appendix}\label{sec:appendix}

\subsubsection{subsection}
\begin{figure}[h]
	\centering
	\includegraphics[width=8.9cm]{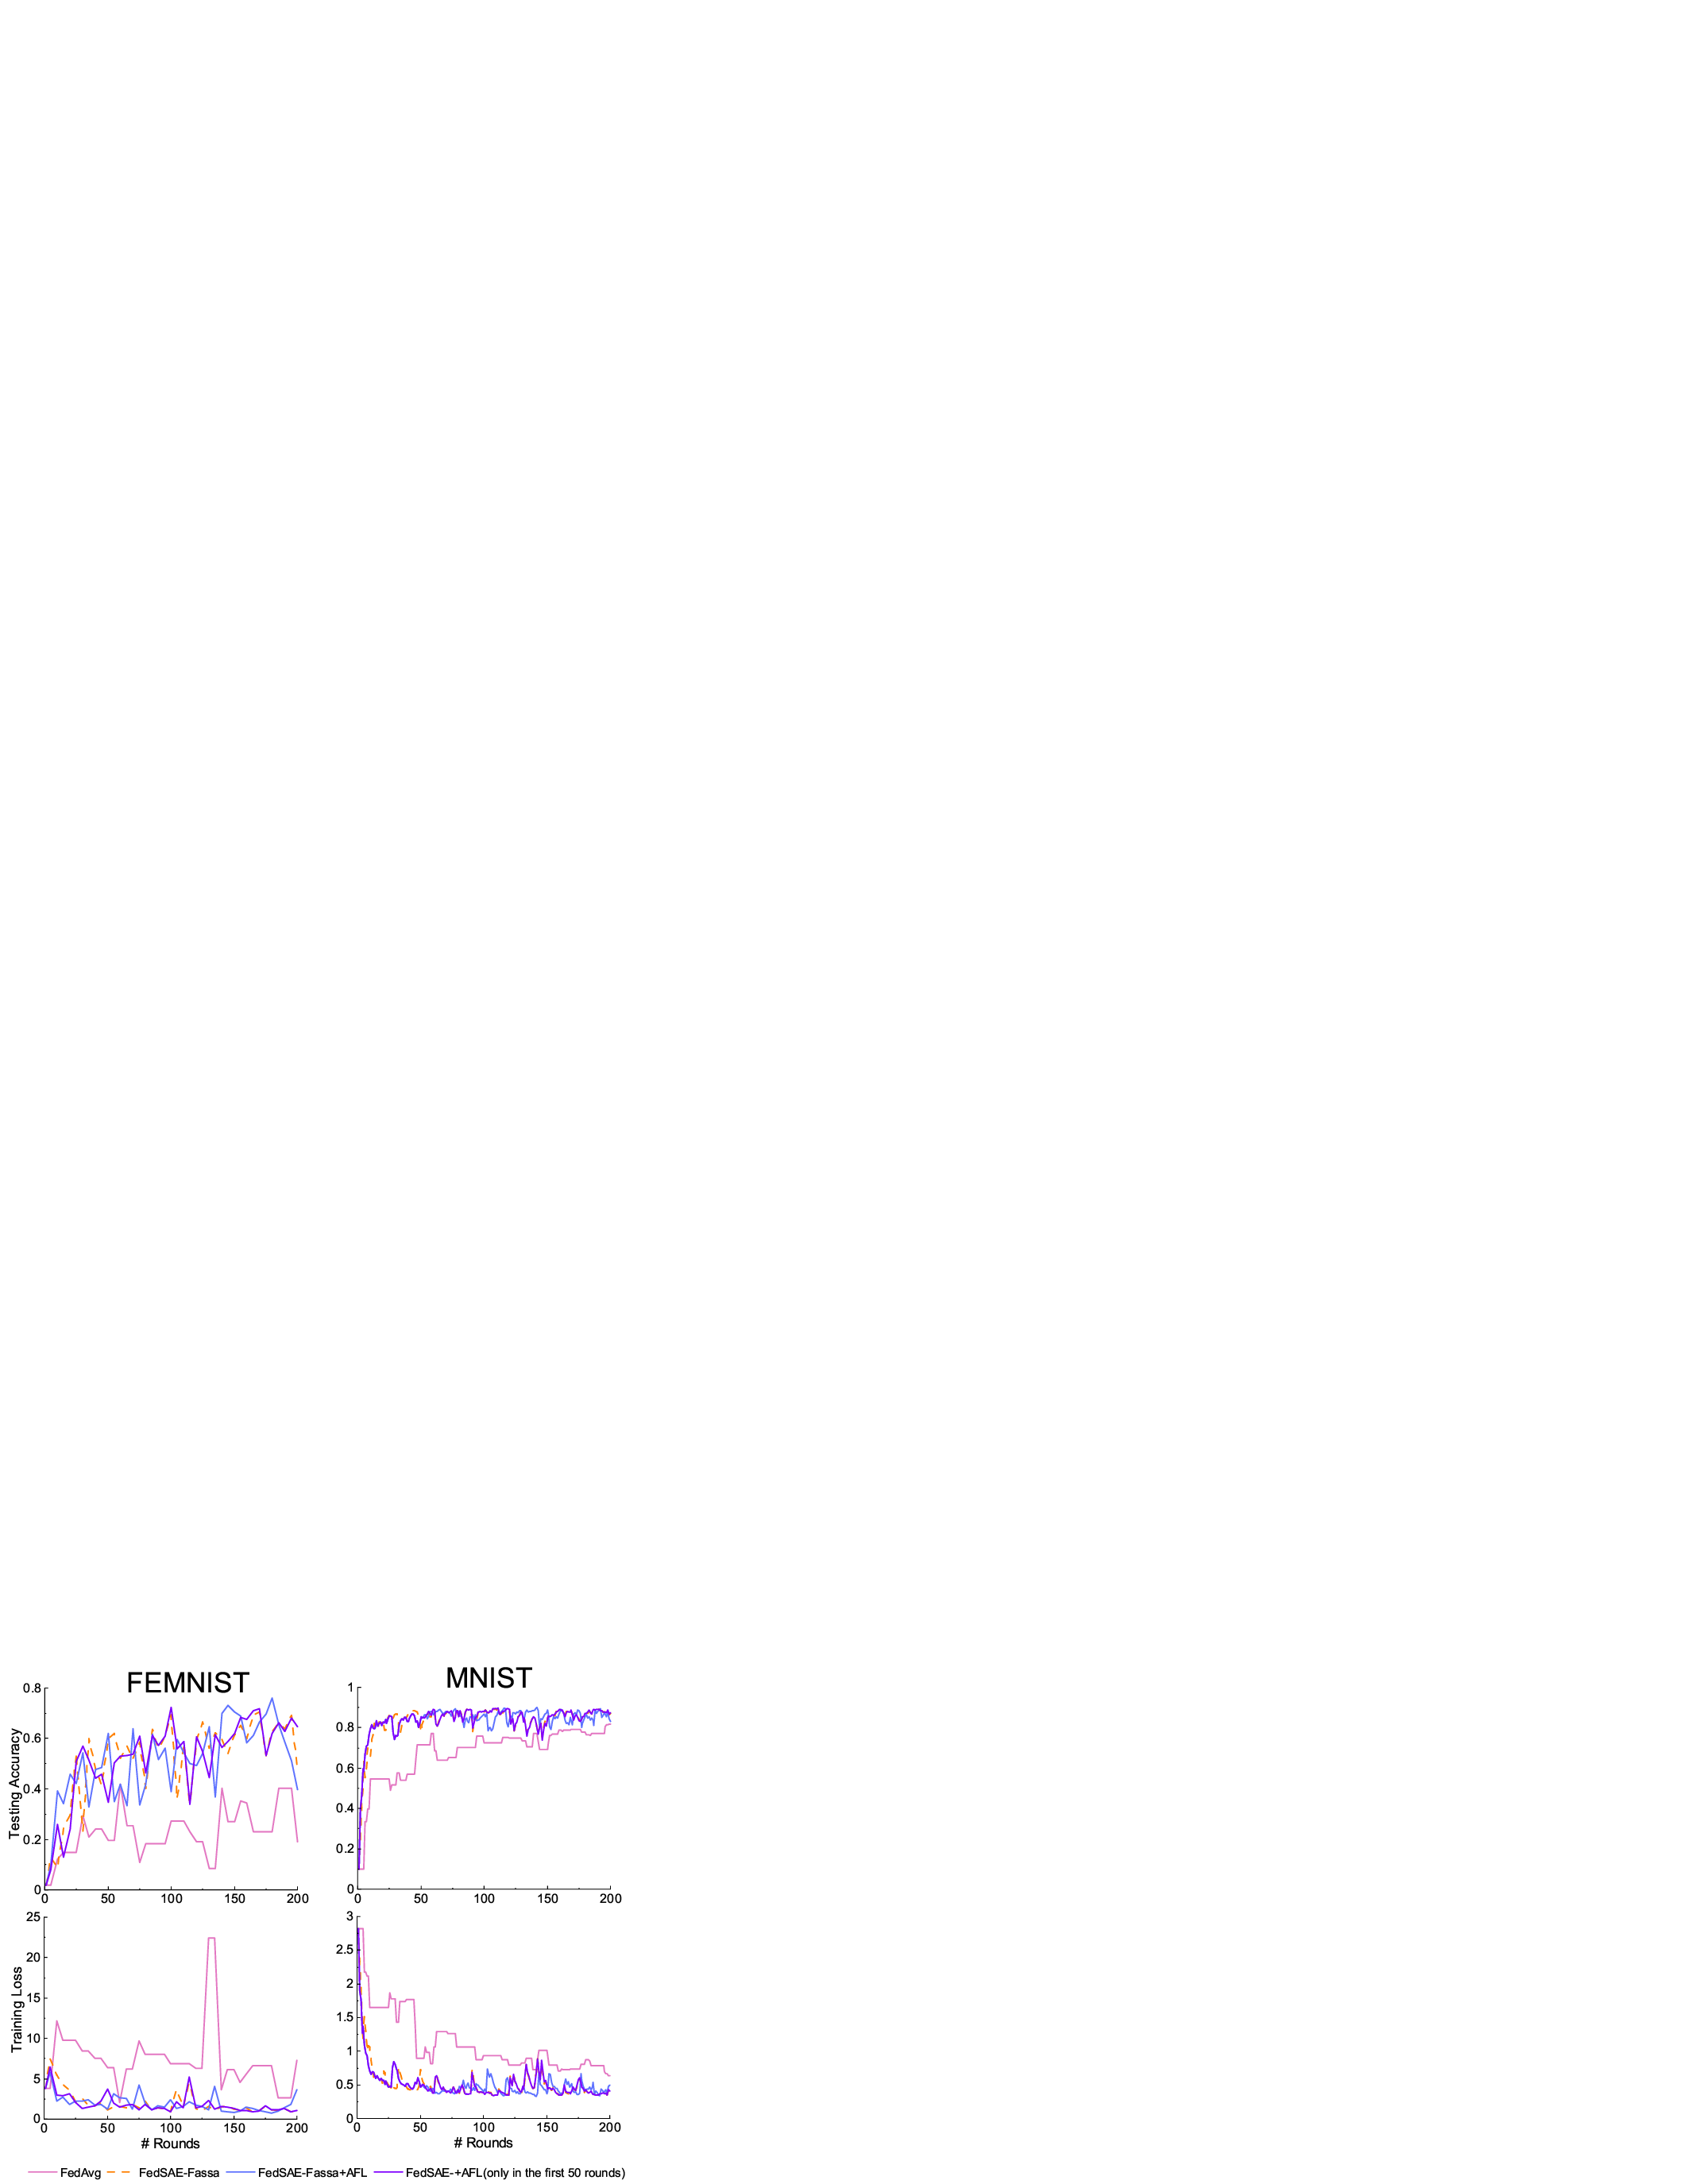}
	\caption{{FedSAE-Fassa} further combined with AFL accelerates convergence too contrast with \textit{FedAvg} and original \textit{FedSAE-Fassa}.}
	\label{fig:Fassa-AFL}
\end{figure}
